# Supplementary material for: Analytic energy gradients for variational two-electron reduced-density matrix methods within the density-fitting approximation
Source: arXiv:1809.09058 ancillary file (2018-11-28)
Supplement: Supplementary file 1 [file si.pdf]

# Supporting information for: Analytic energy gradients for variational two-electron reduced-density matrix methods within the density-fitting approximation

J. Wayne Mullinax,[†] Evgeny Epifanovsky,[‡] Gergely Gidofalvi,[¶] and A. Eugene DePrince III[*,†]

† *Department of Chemistry and Biochemistry, Florida State University, Tallahassee, FL 32306*

‡ *Q-Chem, Inc., 6601 Owens Drive, Suite 105, Pleasanton, CA 94588*

¶ *Department of Chemistry and Biochemistry, Gonzaga University, Spokane, Washington 99258*

E-mail: deprince@chem.fsu.edu

# 1 Convergence criteria for harmonic frequencies

Table S1 reports harmonic frequencies determined from full-valence v2RDM-CASSCF computations performed under the PQG $N$-representability conditions (labeled simply as "PQG" below) using two different sets of convergence criteria. All computations used the cc-pVDZ basis set and the cc-pVDZ-JK auxiliary basis set. Four convergence thresholds enter a v2RDM-CASSCF gradient calculation; these thresholds are defined in the main text of the manuscript. The "tight" convergence criteria require $\epsilon_{\text{error}} < 1.0 \times 10^{-8}$, $\epsilon_{\text{gap}} < 1.0 \times 10^{-8}$ $E_{\text{h}}$, $\epsilon_{\text{ograd}} < 1.0 \times 10^{-8}$ $E_{\text{h}}$, and $\epsilon_{\text{oene}} < 1.0 \times 10^{-11}$ $E_{\text{h}}$. The "loose" convergence criteria require $\epsilon_{\text{error}} < 1.0 \times 10^{-6}$, $\epsilon_{\text{gap}} < 1.0 \times 10^{-6}$ $E_{\text{h}}$, $\epsilon_{\text{ograd}} < 1.0 \times 10^{-6}$ $E_{\text{h}}$, and $\epsilon_{\text{oene}} < 1.0 \times 10^{-9}$ $E_{\text{h}}$. For frequencies evaluated under both criteria, the only significant discrepancy that arises is for the $\Pi$ bending mode of HNC, where the loose criteria yield a frequency that is 67 cm$^{-1}$ lower than that obtained from tightly converged computations. All other frequency differences are less than 2 cm$^{-1}$.

Table S1: Harmonic frequencies from PQG computations that employed "tight" convergence criteria ($\omega_{\text{tight}}$) and the deviation from $\omega_{\text{tight}}$ observed when using "loose" convergence criteria ($\delta\omega_{\text{loose}}$).

| Molecule | Term | Mode | Sym | $\omega_{\text{tight}}$ | $\delta\omega_{\text{loose}}$ |
|---|---|---|---|---|---|
| BF | $^1\Sigma^+$ | 1 | Σ | 1334.1 | 0.0 |
| BH | $^1\Sigma^+$ | 1 | Σ | 2227.5 | 0.0 |
| $C_2$ | $^1\Sigma_g^+$ | 1 | $\Sigma_g$ | 1491.9 | −0.1 |
| $CH_2$ | $^1A_1$ | 1 | $A_1$ | 2760.7 | −0.2 |
| | | 2 | $A_1$ | 1361.6 | 0.3 |
| | | 3 | $B_2$ | 2846.3 | 0.0 |
| $CH_4$ | $^1A_1$ | 1 | $A_1$ | 2883.1 | −0.3 |
| | | 2 | E | 1525.0 | 0.0 |
| | | 3 | $T_2$ | 3085.4 | 0.0 |
| | | 4 | $T_2$ | 1330.9 | −0.2 |
| CO | $^1\Sigma^+$ | 1 | Σ | 2126.3 | 0.0 |
| $F_2$ | $^1\Sigma_g^+$ | 1 | $\Sigma_g$ | 612.0 | 0.0 |
| $H_2O$ | $^1A_1$ | 1 | $A_1$ | 3699.0 | 0.1 |
| | | 2 | $A_1$ | 1709.1 | 0.0 |
| | | 3 | $B_2$ | 3810.9 | 0.0 |
| HCN | $^1\Sigma^+$ | 1 | Σ | 3319.0 | −0.1 |
| | | 2 | Σ | 2024.1 | 0.3 |
| | | 3 | Π | 605.4 | 0.3 |
| HF | $^1\Sigma^+$ | 1 | Σ | 4055.4 | −0.8 |
| HNC | $^1\Sigma^+$ | 1 | Σ | 3639.2 | 0.0 |
| | | 2 | Σ | 1970.0 | −0.1 |
| | | 3 | Π | 231.6 | −67.0 |
| HNO | $^1A'$ | 1 | A′ | 2657.7 | 0.9 |
| | | 2 | A′ | 1580.7 | −0.4 |
| | | 3 | A′ | 1542.7 | 0.0 |
| HOF | $^1A'$ | 1 | A′ | 3624.9 | 0.0 |
| | | 2 | A′ | 1313.1 | −0.3 |
| | | 3 | A′ | 735.9 | 0.0 |
| $N_2$ | $^1\Sigma_g^+$ | 1 | $\Sigma_g$ | 2304.8 | 0.1 |
| $N_2H_2$ | $^1A_g$ | 1 | $A_g$ | 2993.0 | 0.2 |
| | | 2 | $A_g$ | 1613.2 | −1.2 |
| | | 3 | $A_g$ | 1544.9 | 0.3 |
| | | 4 | $A_u$ | 1278.8 | 0.0 |
| | | 5 | $B_u$ | 3047.5 | 0.0 |
| | | 6 | $B_u$ | 1344.1 | 0.0 |
| $NH_3$ | $^1A_1$ | 1 | $A_1$ | 3285.1 | 0.1 |
| | | 2 | $A_1$ | 1207.3 | 1.8 |
| | | 3 | E | 3426.3 | 0.1 |
| | | 4 | E | 1688.6 | 0.0 |
| BO | $^2\Sigma^+$ | 1 | Σ | 1824.9 | −0.1 |
| CH | $^2\Pi$ | 1 | Σ | 2775.3 | −0.3 |
| $NH_2$ | $^2B_1$ | 1 | $A_1$ | 3189.4 | 0.3 |
| | | 2 | $A_1$ | 1565.1 | −0.8 |
| | | 3 | $B_2$ | 3281.8 | 0.1 |
| OH | $^2\Pi$ | 1 | Σ | 3607.6 | 0.0 |
| $B_2$ | $^3\Sigma_g^-$ | 1 | $\Sigma_g$ | 878.0 | 0.0 |
| $CH_2$ | $^3B_1$ | 1 | $A_1$ | 3023.8 | 0.0 |
| | | 2 | $A_1$ | 1156.5 | 0.0 |
| | | 3 | $B_2$ | 3231.6 | 0.0 |
| NF | $^3\Sigma^-$ | 1 | Σ | 1074.3 | −0.1 |
| NH | $^3\Sigma^-$ | 1 | Σ | 3110.9 | 0.1 |
| $O_2$ | $^3\Sigma_g^-$ | 1 | $\Sigma_g$ | 1472.6 | 0.0 |

## 2 Bond Length Alternation

Tables S2-S10 report the bond lengths along the long axis of the singlet and triplet states of the linear polyacene series (naphthalene through dodecacene). Equilibrium geometries were obtained from PQG computations using the the cc-pVDZ basis set and the cc-pVDZ-JK auxiliary basis set. The convergence criteria employed in the computations are reported in the main text of the manuscript. These results indicate that the PQG-derived equilibrium geometries of the singlet and triplet states become more similar as the length of the acene molecule increases.

Table S2: Bond lengths (Å) along the long axis of naphthalene in its singlet and triplet states.

| Bond | Singlet | Triplet | Difference |
|---|---|---|---|
| 1 | 1.383 | 1.437 | -0.054 |
| 2 | 1.423 | 1.417 | 0.006 |
| 3 | 1.423 | 1.417 | 0.006 |
| 4 | 1.383 | 1.437 | -0.054 |

Table S3: Bond lengths (Å) along the long axis of anthracene in its singlet and triplet states.

| Bond | Singlet | Triplet | Difference |
|---|---|---|---|
| 1 | 1.378 | 1.417 | -0.039 |
| 2 | 1.430 | 1.409 | 0.021 |
| 3 | 1.406 | 1.425 | -0.019 |
| 4 | 1.406 | 1.425 | -0.019 |
| 5 | 1.430 | 1.409 | 0.021 |
| 6 | 1.378 | 1.417 | -0.039 |

Table S4: Bond lengths (Å) along the long axis of tetracene in its singlet and triplet states.

| Bond | Singlet | Triplet | Difference |
|---|---|---|---|
| 1 | 1.378 | 1.404 | -0.026 |
| 2 | 1.431 | 1.413 | 0.019 |
| 3 | 1.403 | 1.425 | -0.022 |
| 4 | 1.413 | 1.412 | 0.002 |
| 5 | 1.413 | 1.412 | 0.002 |
| 6 | 1.403 | 1.425 | -0.022 |
| 7 | 1.431 | 1.413 | 0.019 |
| 8 | 1.378 | 1.404 | -0.026 |

Table S5: Bond lengths (Å) along the long axis of pentacene in its singlet and triplet states.

| Bond | Singlet | Triplet | Difference |
|---|---|---|---|
| 1 | 1.379 | 1.395 | -0.016 |
| 2 | 1.430 | 1.417 | 0.013 |
| 3 | 1.404 | 1.421 | -0.017 |
| 4 | 1.414 | 1.407 | 0.007 |
| 5 | 1.410 | 1.417 | -0.006 |
| 6 | 1.410 | 1.417 | -0.006 |
| 7 | 1.414 | 1.407 | 0.007 |
| 8 | 1.404 | 1.421 | -0.017 |
| 9 | 1.430 | 1.417 | 0.013 |
| 10 | 1.379 | 1.395 | -0.016 |

Table S6: Bond lengths (Å) along the long axis of hexacene in its singlet and triplet states.

| Bond | Singlet | Triplet | Difference |
|---|---|---|---|
| 1 | 1.381 | 1.391 | -0.010 |
| 2 | 1.429 | 1.420 | 0.008 |
| 3 | 1.406 | 1.417 | -0.011 |
| 4 | 1.413 | 1.407 | 0.006 |
| 5 | 1.412 | 1.418 | -0.006 |
| 6 | 1.411 | 1.411 | -0.000 |
| 7 | 1.411 | 1.411 | -0.000 |
| 8 | 1.412 | 1.418 | -0.006 |
| 9 | 1.413 | 1.407 | 0.006 |
| 10 | 1.406 | 1.417 | -0.011 |
| 11 | 1.429 | 1.420 | 0.008 |
| 12 | 1.381 | 1.391 | -0.010 |

Table S7: Bond lengths (Å) along the long axis of heptacene in its singlet and triplet states.

| Bond | Singlet | Triplet | Difference |
|---|---|---|---|
| 1 | 1.382 | 1.388 | -0.006 |
| 2 | 1.428 | 1.422 | 0.005 |
| 3 | 1.408 | 1.415 | -0.007 |
| 4 | 1.411 | 1.408 | 0.003 |
| 5 | 1.413 | 1.417 | -0.004 |
| 6 | 1.410 | 1.409 | 0.000 |
| 7 | 1.412 | 1.414 | -0.002 |
| 8 | 1.412 | 1.414 | -0.002 |
| 9 | 1.410 | 1.409 | 0.000 |
| 10 | 1.413 | 1.417 | -0.004 |
| 11 | 1.411 | 1.408 | 0.003 |
| 12 | 1.408 | 1.415 | -0.007 |
| 13 | 1.428 | 1.422 | 0.005 |
| 14 | 1.382 | 1.388 | -0.006 |

Table S8: Bond lengths (Å) along the long axis of octacene in its singlet and triplet states.

| Bond | Singlet | Triplet | Difference |
|---|---|---|---|
| 1 | 1.382 | 1.386 | -0.004 |
| 2 | 1.427 | 1.424 | 0.003 |
| 3 | 1.408 | 1.413 | -0.005 |
| 4 | 1.410 | 1.409 | 0.002 |
| 5 | 1.415 | 1.417 | -0.002 |
| 6 | 1.408 | 1.409 | -0.001 |
| 7 | 1.414 | 1.414 | -0.001 |
| 8 | 1.410 | 1.411 | -0.001 |
| 9 | 1.410 | 1.411 | -0.001 |
| 10 | 1.414 | 1.414 | -0.001 |
| 11 | 1.408 | 1.409 | -0.001 |
| 12 | 1.415 | 1.417 | -0.002 |
| 13 | 1.410 | 1.409 | 0.002 |
| 14 | 1.408 | 1.413 | -0.005 |
| 15 | 1.427 | 1.424 | 0.003 |
| 16 | 1.382 | 1.386 | -0.004 |

Table S9: Bond lengths (Å) along the long axis of nonacene in its singlet and triplet states.

| Bond | Singlet | Triplet | Difference |
|---|---|---|---|
| 1 | 1.382 | 1.385 | -0.003 |
| 2 | 1.427 | 1.425 | 0.003 |
| 3 | 1.409 | 1.412 | -0.003 |
| 4 | 1.410 | 1.409 | 0.001 |
| 5 | 1.415 | 1.416 | -0.001 |
| 6 | 1.407 | 1.409 | -0.001 |
| 7 | 1.414 | 1.414 | 0.001 |
| 8 | 1.409 | 1.411 | -0.002 |
| 9 | 1.412 | 1.412 | -0.000 |
| 10 | 1.412 | 1.412 | -0.000 |
| 11 | 1.409 | 1.411 | -0.002 |
| 12 | 1.414 | 1.414 | 0.001 |
| 13 | 1.407 | 1.409 | -0.001 |
| 14 | 1.415 | 1.416 | -0.001 |
| 15 | 1.410 | 1.409 | 0.001 |
| 16 | 1.409 | 1.412 | -0.003 |
| 17 | 1.427 | 1.425 | 0.003 |
| 18 | 1.382 | 1.385 | -0.003 |

Table S10: Bond lengths (Å) along the long axis of decacene in its singlet and triplet states.

| Bond | Singlet | Triplet | Difference |
|---|---|---|---|
| 1 | 1.382 | 1.384 | -0.002 |
| 2 | 1.427 | 1.425 | 0.002 |
| 3 | 1.408 | 1.411 | -0.003 |
| 4 | 1.410 | 1.409 | 0.001 |
| 5 | 1.415 | 1.416 | -0.001 |
| 6 | 1.407 | 1.409 | -0.001 |
| 7 | 1.415 | 1.414 | 0.001 |
| 8 | 1.408 | 1.411 | -0.002 |
| 9 | 1.413 | 1.412 | 0.001 |
| 10 | 1.411 | 1.412 | -0.001 |
| 11 | 1.411 | 1.412 | -0.001 |
| 12 | 1.413 | 1.412 | 0.001 |
| 13 | 1.408 | 1.411 | -0.002 |
| 14 | 1.415 | 1.414 | 0.001 |
| 15 | 1.407 | 1.409 | -0.001 |
| 16 | 1.415 | 1.416 | -0.001 |
| 17 | 1.410 | 1.409 | 0.001 |
| 18 | 1.408 | 1.411 | -0.003 |
| 19 | 1.427 | 1.425 | 0.002 |
| 20 | 1.382 | 1.384 | -0.002 |

Table S11: Bond lengths (Å) along the long axis of undecacene in its singlet and triplet states.

| Bond | Singlet | Triplet | Difference |
|---|---|---|---|
| 1 | 1.382 | 1.384 | -0.002 |
| 2 | 1.427 | 1.425 | 0.002 |
| 3 | 1.408 | 1.411 | -0.002 |
| 4 | 1.410 | 1.409 | 0.001 |
| 5 | 1.415 | 1.416 | -0.001 |
| 6 | 1.407 | 1.408 | -0.001 |
| 7 | 1.415 | 1.414 | 0.001 |
| 8 | 1.408 | 1.411 | -0.002 |
| 9 | 1.413 | 1.412 | 0.001 |
| 10 | 1.410 | 1.412 | -0.002 |
| 11 | 1.411 | 1.412 | -0.000 |
| 12 | 1.411 | 1.412 | -0.000 |
| 13 | 1.410 | 1.412 | -0.002 |
| 14 | 1.413 | 1.412 | 0.001 |
| 15 | 1.408 | 1.411 | -0.002 |
| 16 | 1.415 | 1.414 | 0.001 |
| 17 | 1.407 | 1.408 | -0.001 |
| 18 | 1.415 | 1.416 | -0.001 |
| 19 | 1.410 | 1.409 | 0.001 |
| 20 | 1.408 | 1.411 | -0.002 |
| 21 | 1.427 | 1.425 | 0.002 |
| 22 | 1.382 | 1.384 | -0.002 |

Table S12: Bond lengths (Å) along the long axis of dodecacene in its singlet and triplet states.

| Bond | Singlet | Triplet | Difference |
|---|---|---|---|
| 1 | 1.382 | 1.384 | -0.002 |
| 2 | 1.427 | 1.426 | 0.002 |
| 3 | 1.408 | 1.410 | -0.002 |
| 4 | 1.410 | 1.409 | 0.001 |
| 5 | 1.415 | 1.416 | -0.001 |
| 6 | 1.407 | 1.408 | -0.001 |
| 7 | 1.415 | 1.414 | 0.001 |
| 8 | 1.408 | 1.410 | -0.002 |
| 9 | 1.413 | 1.412 | 0.001 |
| 10 | 1.410 | 1.412 | -0.002 |
| 11 | 1.412 | 1.411 | 0.001 |
| 12 | 1.411 | 1.412 | -0.001 |
| 13 | 1.411 | 1.412 | -0.001 |
| 14 | 1.412 | 1.411 | 0.001 |
| 15 | 1.410 | 1.412 | -0.002 |
| 16 | 1.413 | 1.412 | 0.001 |
| 17 | 1.408 | 1.410 | -0.002 |
| 18 | 1.415 | 1.414 | 0.001 |
| 19 | 1.407 | 1.408 | -0.001 |
| 20 | 1.415 | 1.416 | -0.001 |
| 21 | 1.410 | 1.409 | 0.001 |
| 22 | 1.408 | 1.410 | -0.002 |
| 23 | 1.427 | 1.426 | 0.002 |
| 24 | 1.382 | 1.384 | -0.002 |

# 3 Equilibrium geometries of the linear acenes

This Section provides the Cartesian coordinates for the equilibrium geometries of the acene molecules in the singlet and triplet spin states, which were optimized the PQG/cc-pVDZ level of theory. The auxiliary basis set employed within the density fitting approximation was cc-pVDZ-JK. The active space consisted of the $\pi$ valence orbitals. The convergence criteria are reported in the main text of the manuscript.

**naphthalene (singlet)**

```
18
Energy: -383.53523 hartree
  C      2.4400897185      0.7094315040      0.0000000000
  C      1.2450334016      1.4046515440      0.0000000000
  C      0.0000000000      0.7152967835      0.0000000000
  C     -1.2450334016      1.4046515440      0.0000000000
  C     -2.4400897185      0.7094315040      0.0000000000
  C      2.4400897185     -0.7094315040      0.0000000000
  C      1.2450334016     -1.4046515440      0.0000000000
  C      0.0000000000     -0.7152967835      0.0000000000
  C     -1.2450334016     -1.4046515440      0.0000000000
  C     -2.4400897185     -0.7094315040      0.0000000000
  H      3.3796489895      1.2457068567      0.0000000000
  H      1.2452445840      2.4870605918      0.0000000000
  H     -1.2452445840      2.4870605918      0.0000000000
  H     -3.3796489895      1.2457068567      0.0000000000
  H      3.3796489895     -1.2457068567      0.0000000000
  H      1.2452445840     -2.4870605918      0.0000000000
  H     -1.2452445840     -2.4870605918      0.0000000000
  H     -3.3796489895     -1.2457068567      0.0000000000
```

**naphthalene (triplet)**

```
18
Energy: -383.43584 hartree
  C      2.4863732564      0.6898102668      0.0000000000
  C      1.2413393053      1.4071472955      0.0000000000
  C      0.0000000000      0.7236002940      0.0000000000
  C     -1.2413393053      1.4071472955      0.0000000000
  C     -2.4863732564      0.6898102668      0.0000000000
  C      2.4863732564     -0.6898102668      0.0000000000
  C      1.2413393053     -1.4071472955      0.0000000000
  C      0.0000000000     -0.7236002940      0.0000000000
```

| | | | |
|---|---|---|---|
| C | -1.2413393053 | -1.4071472955 | 0.0000000000 |
| C | -2.4863732564 | -0.6898102668 | 0.0000000000 |
| H | 3.4163700581 | 1.2413152245 | 0.0000000000 |
| H | 1.2491827644 | 2.4886094242 | 0.0000000000 |
| H | -1.2491827644 | 2.4886094242 | 0.0000000000 |
| H | -3.4163700581 | 1.2413152245 | 0.0000000000 |
| H | 3.4163700581 | -1.2413152245 | 0.0000000000 |
| H | 1.2491827644 | -2.4886094242 | 0.0000000000 |
| H | -1.2491827644 | -2.4886094242 | 0.0000000000 |
| H | -3.4163700581 | -1.2413152245 | 0.0000000000 |

**anthracene (singlet)**

24
Energy: -536.26064 hartree

| | | | |
|---|---|---|---|
| C | 3.6712956303 | 0.7133112028 | 0.0000000000 |
| C | 2.4813222907 | 1.4082353907 | 0.0000000000 |
| C | 1.2279831276 | 0.7197194532 | 0.0000000000 |
| C | 0.0000000000 | 1.4054725778 | 0.0000000000 |
| C | -1.2279831276 | 0.7197194532 | 0.0000000000 |
| C | -2.4813222907 | 1.4082353907 | 0.0000000000 |
| C | -3.6712956303 | 0.7133112028 | 0.0000000000 |
| C | 3.6712956303 | -0.7133112028 | 0.0000000000 |
| C | 2.4813222907 | -1.4082353907 | 0.0000000000 |
| C | 1.2279831276 | -0.7197194532 | 0.0000000000 |
| C | 0.0000000000 | -1.4054725778 | 0.0000000000 |
| C | -1.2279831276 | -0.7197194532 | 0.0000000000 |
| C | -2.4813222907 | -1.4082353907 | 0.0000000000 |
| C | -3.6712956303 | -0.7133112028 | 0.0000000000 |
| H | 4.6120166452 | 1.2473323697 | 0.0000000000 |
| H | 2.4819044211 | 2.4905029907 | 0.0000000000 |
| H | 0.0000000000 | 2.4880580140 | 0.0000000000 |
| H | -2.4819044211 | 2.4905029907 | 0.0000000000 |
| H | -4.6120166452 | 1.2473323697 | 0.0000000000 |
| H | 4.6120166452 | -1.2473323697 | 0.0000000000 |
| H | 2.4819044211 | -2.4905029907 | 0.0000000000 |
| H | 0.0000000000 | -2.4880580140 | 0.0000000000 |
| H | -2.4819044211 | -2.4905029907 | 0.0000000000 |
| H | -4.6120166452 | -1.2473323697 | 0.0000000000 |

**anthracene (triplet)**

24
Energy: -536.19078 hartree

| | | | |
|---|---|---|---|
| C | 3.7093105268 | 0.6958028488 | 0.0000000000 |
| C | 2.4817280469 | 1.4031752030 | 0.0000000000 |

```
  C      1.2488828020      0.7201754015      0.0000000000
  C      0.0000000000      1.4072012474      0.0000000000
  C     -1.2488828020      0.7201754015      0.0000000000
  C     -2.4817280469      1.4031752030      0.0000000000
  C     -3.7093105268      0.6958028488      0.0000000000
  C      3.7093105268     -0.6958028488      0.0000000000
  C      2.4817280469     -1.4031752030      0.0000000000
  C      1.2488828020     -0.7201754015      0.0000000000
  C      0.0000000000     -1.4072012474      0.0000000000
  C     -1.2488828020     -0.7201754015      0.0000000000
  C     -2.4817280469     -1.4031752030      0.0000000000
  C     -3.7093105268     -0.6958028488      0.0000000000
  H      4.6421699246      1.2427605764      0.0000000000
  H      2.4868224805      2.4851363569      0.0000000000
  H      0.0000000000      2.4893028532      0.0000000000
  H     -2.4868224805      2.4851363569      0.0000000000
  H     -4.6421699246      1.2427605764      0.0000000000
  H      4.6421699246     -1.2427605764      0.0000000000
  H      2.4868224805     -2.4851363569      0.0000000000
  H      0.0000000000     -2.4893028532      0.0000000000
  H     -2.4868224805     -2.4851363569      0.0000000000
  H     -4.6421699246     -1.2427605764      0.0000000000
```

**tetracene (singlet)**

```
30
Energy: -688.98535 hartree
  C      4.9052018440      0.7140740300      0.0000000000
  C      3.7155081006      1.4092843941      0.0000000000
  C      2.4604058560      0.7216908514      0.0000000000
  C      1.2364280970      1.4076141609      0.0000000000
  C      0.0000000000      0.7226723786      0.0000000000
  C     -1.2364280970      1.4076141609      0.0000000000
  C     -2.4604058560      0.7216908514      0.0000000000
  C     -3.7155081006      1.4092843941      0.0000000000
  C     -4.9052018440      0.7140740300      0.0000000000
  C      4.9052018440     -0.7140740300      0.0000000000
  C      3.7155081006     -1.4092843941      0.0000000000
  C      2.4604058560     -0.7216908514      0.0000000000
  C      1.2364280970     -1.4076141609      0.0000000000
  C      0.0000000000     -0.7226723786      0.0000000000
  C     -1.2364280970     -1.4076141609      0.0000000000
  C     -2.4604058560     -0.7216908514      0.0000000000
  C     -3.7155081006     -1.4092843941      0.0000000000
  C     -4.9052018440     -0.7140740300      0.0000000000
  H      5.8460324004      1.2478014938      0.0000000000
```

```
  H      3.7164676499      2.4915189212      0.0000000000
  H      1.2368453762      2.4900419700      0.0000000000
  H     -1.2368453762      2.4900419700      0.0000000000
  H     -3.7164676499      2.4915189212      0.0000000000
  H     -5.8460324004      1.2478014938      0.0000000000
  H      5.8460324004     -1.2478014938      0.0000000000
  H      3.7164676499     -2.4915189212      0.0000000000
  H      1.2368453762     -2.4900419700      0.0000000000
  H     -1.2368453762     -2.4900419700      0.0000000000
  H     -3.7164676499     -2.4915189212      0.0000000000
  H     -5.8460324004     -1.2478014938      0.0000000000
```

**tetracene (triplet)**

```
30
Energy: -688.93549 hartree
  C      4.9346562269      0.7010105834      0.0000000000
  C      3.7193981455      1.4033045340      0.0000000000
  C      2.4839727811      0.7184476992      0.0000000000
  C      1.2358921748      1.4064366770      0.0000000000
  C      0.0000000000      0.7237713145      0.0000000000
  C     -1.2358921748      1.4064366770      0.0000000000
  C     -2.4839727811      0.7184476992      0.0000000000
  C     -3.7193981455      1.4033045340      0.0000000000
  C     -4.9346562269      0.7010105834      0.0000000000
  C      4.9346562269     -0.7010105834      0.0000000000
  C      3.7193981455     -1.4033045340      0.0000000000
  C      2.4839727811     -0.7184476992      0.0000000000
  C      1.2358921748     -1.4064366770      0.0000000000
  C      0.0000000000     -0.7237713145      0.0000000000
  C     -1.2358921748     -1.4064366770      0.0000000000
  C     -2.4839727811     -0.7184476992      0.0000000000
  C     -3.7193981455     -1.4033045340      0.0000000000
  C     -4.9346562269     -0.7010105834      0.0000000000
  H      5.8699168909      1.2440551505      0.0000000000
  H      3.7226183370      2.4854379510      0.0000000000
  H      1.2373584031      2.4886790585      0.0000000000
  H     -1.2373584031      2.4886790585      0.0000000000
  H     -3.7226183370      2.4854379510      0.0000000000
  H     -5.8699168909      1.2440551505      0.0000000000
  H      5.8699168909     -1.2440551505      0.0000000000
  H      3.7226183370     -2.4854379510      0.0000000000
  H      1.2373584031     -2.4886790585      0.0000000000
  H     -1.2373584031     -2.4886790585      0.0000000000
  H     -3.7226183370     -2.4854379510      0.0000000000
  H     -5.8699168909     -1.2440551505      0.0000000000
```

**pentacene (singlet)**

```
36
Energy: -841.71071 hartree
  C      6.1405742383      0.7136267901      0.0000000000
  C      4.9495666675      1.4091775807      0.0000000000
  C      3.6954690232      0.7219202147      0.0000000000
  C      2.4705825544      1.4081011335      0.0000000000
  C      1.2328617337      0.7241366572      0.0000000000
  C      0.0000000000      1.4092652260      0.0000000000
  C     -1.2328617337      0.7241366572      0.0000000000
  C     -2.4705825544      1.4081011335      0.0000000000
  C     -3.6954690232      0.7219202147      0.0000000000
  C     -4.9495666675      1.4091775807      0.0000000000
  C     -6.1405742383      0.7136267901      0.0000000000
  C      6.1405742383     -0.7136267901      0.0000000000
  C      4.9495666675     -1.4091775807      0.0000000000
  C      3.6954690232     -0.7219202147      0.0000000000
  C      2.4705825544     -1.4081011335      0.0000000000
  C      1.2328617337     -0.7241366572      0.0000000000
  C      0.0000000000     -1.4092652260      0.0000000000
  C     -1.2328617337     -0.7241366572      0.0000000000
  C     -2.4705825544     -1.4081011335      0.0000000000
  C     -3.6954690232     -0.7219202147      0.0000000000
  C     -4.9495666675     -1.4091775807      0.0000000000
  C     -6.1405742383     -0.7136267901      0.0000000000
  H      7.0811305053      1.2477794220      0.0000000000
  H      4.9506989413      2.4914055690      0.0000000000
  H      2.4713678737      2.4905000089      0.0000000000
  H      0.0000000000      2.4915333585      0.0000000000
  H     -2.4713678737      2.4905000089      0.0000000000
  H     -4.9506989413      2.4914055690      0.0000000000
  H     -7.0811305053      1.2477794220      0.0000000000
  H      7.0811305053     -1.2477794220      0.0000000000
  H      4.9506989413     -2.4914055690      0.0000000000
  H      2.4713678737     -2.4905000089      0.0000000000
  H      0.0000000000     -2.4915333585      0.0000000000
  H     -2.4713678737     -2.4905000089      0.0000000000
  H     -4.9506989413     -2.4914055690      0.0000000000
  H     -7.0811305053     -1.2477794220      0.0000000000
```

**pentacene (triplet)**

```
36
Energy: -841.67397 hartree
  C      6.1624762366      0.7047424977      0.0000000000
```

| | | | |
|---|---|---|---|
| C | 4.9551271285 | 1.4044091907 | 0.0000000000 |
| C | 3.7154599755 | 0.7183632742 | 0.0000000000 |
| C | 2.4716592395 | 1.4060616468 | 0.0000000000 |
| C | 1.2407853246 | 0.7236217194 | 0.0000000000 |
| C | 0.0000000000 | 1.4077227389 | 0.0000000000 |
| C | -1.2407853246 | 0.7236217194 | 0.0000000000 |
| C | -2.4716592395 | 1.4060616468 | 0.0000000000 |
| C | -3.7154599755 | 0.7183632742 | 0.0000000000 |
| C | -4.9551271285 | 1.4044091907 | 0.0000000000 |
| C | -6.1624762366 | 0.7047424977 | 0.0000000000 |
| C | 6.1624762366 | -0.7047424977 | 0.0000000000 |
| C | 4.9551271285 | -1.4044091907 | 0.0000000000 |
| C | 3.7154599755 | -0.7183632742 | 0.0000000000 |
| C | 2.4716592395 | -1.4060616468 | 0.0000000000 |
| C | 1.2407853246 | -0.7236217194 | 0.0000000000 |
| C | 0.0000000000 | -1.4077227389 | 0.0000000000 |
| C | -1.2407853246 | -0.7236217194 | 0.0000000000 |
| C | -2.4716592395 | -1.4060616468 | 0.0000000000 |
| C | -3.7154599755 | -0.7183632742 | 0.0000000000 |
| C | -4.9551271285 | -1.4044091907 | 0.0000000000 |
| C | -6.1624762366 | -0.7047424977 | 0.0000000000 |
| H | 7.0993841706 | 1.2450635810 | 0.0000000000 |
| H | 4.9573885835 | 2.4866024101 | 0.0000000000 |
| H | 2.4730709441 | 2.4884037262 | 0.0000000000 |
| H | 0.0000000000 | 2.4899275914 | 0.0000000000 |
| H | -2.4730709441 | 2.4884037262 | 0.0000000000 |
| H | -4.9573885835 | 2.4866024101 | 0.0000000000 |
| H | -7.0993841706 | 1.2450635810 | 0.0000000000 |
| H | 7.0993841706 | -1.2450635810 | 0.0000000000 |
| H | 4.9573885835 | -2.4866024101 | 0.0000000000 |
| H | 2.4730709441 | -2.4884037262 | 0.0000000000 |
| H | 0.0000000000 | -2.4899275914 | 0.0000000000 |
| H | -2.4730709441 | -2.4884037262 | 0.0000000000 |
| H | -4.9573885835 | -2.4866024101 | 0.0000000000 |
| H | -7.0993841706 | -1.2450635810 | 0.0000000000 |

**hexacene (singlet)**

42
Energy: -994.43705 hartree

| | | | |
|---|---|---|---|
| C | 7.3765336018 | 0.7128562154 | 0.0000000000 |
| C | 6.1840495940 | 1.4086981064 | 0.0000000000 |
| C | 4.9315758863 | 0.7215092560 | 0.0000000000 |
| C | 3.7044808900 | 1.4078910928 | 0.0000000000 |
| C | 2.4682485308 | 0.7242982830 | 0.0000000000 |
| C | 1.2341238547 | 1.4094673900 | 0.0000000000 |

| | | | |
|---|---|---|---|
| C | 0.0000000000 | 0.7254195642 | 0.0000000000 |
| C | -1.2341238547 | 1.4094673900 | 0.0000000000 |
| C | -2.4682485308 | 0.7242982830 | 0.0000000000 |
| C | -3.7044808900 | 1.4078910928 | 0.0000000000 |
| C | -4.9315758863 | 0.7215092560 | 0.0000000000 |
| C | -6.1840495940 | 1.4086981064 | 0.0000000000 |
| C | -7.3765336018 | 0.7128562154 | 0.0000000000 |
| C | 7.3765336018 | -0.7128562154 | 0.0000000000 |
| C | 6.1840495940 | -1.4086981064 | 0.0000000000 |
| C | 4.9315758863 | -0.7215092560 | 0.0000000000 |
| C | 3.7044808900 | -1.4078910928 | 0.0000000000 |
| C | 2.4682485308 | -0.7242982830 | 0.0000000000 |
| C | 1.2341238547 | -1.4094673900 | 0.0000000000 |
| C | 0.0000000000 | -0.7254195642 | 0.0000000000 |
| C | -1.2341238547 | -1.4094673900 | 0.0000000000 |
| C | -2.4682485308 | -0.7242982830 | 0.0000000000 |
| C | -3.7044808900 | -1.4078910928 | 0.0000000000 |
| C | -4.9315758863 | -0.7215092560 | 0.0000000000 |
| C | -6.1840495940 | -1.4086981064 | 0.0000000000 |
| C | -7.3765336018 | -0.7128562154 | 0.0000000000 |
| H | 8.3167572866 | 1.2475665220 | 0.0000000000 |
| H | 6.1852480444 | 2.4909272446 | 0.0000000000 |
| H | 3.7054018275 | 2.4902934902 | 0.0000000000 |
| H | 1.2344616082 | 2.4917193662 | 0.0000000000 |
| H | -1.2344616082 | 2.4917193662 | 0.0000000000 |
| H | -3.7054018275 | 2.4902934902 | 0.0000000000 |
| H | -6.1852480444 | 2.4909272446 | 0.0000000000 |
| H | -8.3167572866 | 1.2475665220 | 0.0000000000 |
| H | 8.3167572866 | -1.2475665220 | 0.0000000000 |
| H | 6.1852480444 | -2.4909272446 | 0.0000000000 |
| H | 3.7054018275 | -2.4902934902 | 0.0000000000 |
| H | 1.2344616082 | -2.4917193662 | 0.0000000000 |
| H | -1.2344616082 | -2.4917193662 | 0.0000000000 |
| H | -3.7054018275 | -2.4902934902 | 0.0000000000 |
| H | -6.1852480444 | -2.4909272446 | 0.0000000000 |
| H | -8.3167572866 | -1.2475665220 | 0.0000000000 |

**hexacene (triplet)**

42

Energy: -994.40857 hartree

| | | | |
|---|---|---|---|
| C | 7.3922892854 | 0.7072059724 | 0.0000000000 |
| C | 6.1897726646 | 1.4054530307 | 0.0000000000 |
| C | 4.9466037317 | 0.7188519591 | 0.0000000000 |
| C | 3.7070241506 | 1.4062198708 | 0.0000000000 |
| C | 2.4767456054 | 0.7232991924 | 0.0000000000 |

| | | | |
|---|---|---|---|
| C | 1.2349594492 | 1.4078761465 | 0.0000000000 |
| C | 0.0000000000 | 0.7246702452 | 0.0000000000 |
| C | -1.2349594492 | 1.4078761465 | 0.0000000000 |
| C | -2.4767456054 | 0.7232991924 | 0.0000000000 |
| C | -3.7070241506 | 1.4062198708 | 0.0000000000 |
| C | -4.9466037317 | 0.7188519591 | 0.0000000000 |
| C | -6.1897726646 | 1.4054530307 | 0.0000000000 |
| C | -7.3922892854 | 0.7072059724 | 0.0000000000 |
| C | 7.3922892854 | -0.7072059724 | 0.0000000000 |
| C | 6.1897726646 | -1.4054530307 | 0.0000000000 |
| C | 4.9466037317 | -0.7188519591 | 0.0000000000 |
| C | 3.7070241506 | -1.4062198708 | 0.0000000000 |
| C | 2.4767456054 | -0.7232991924 | 0.0000000000 |
| C | 1.2349594492 | -1.4078761465 | 0.0000000000 |
| C | 0.0000000000 | -0.7246702452 | 0.0000000000 |
| C | -1.2349594492 | -1.4078761465 | 0.0000000000 |
| C | -2.4767456054 | -0.7232991924 | 0.0000000000 |
| C | -3.7070241506 | -1.4062198708 | 0.0000000000 |
| C | -4.9466037317 | -0.7188519591 | 0.0000000000 |
| C | -6.1897726646 | -1.4054530307 | 0.0000000000 |
| C | -7.3922892854 | -0.7072059724 | 0.0000000000 |
| H | 8.3302360217 | 1.2457864743 | 0.0000000000 |
| H | 6.1915665383 | 2.4876672716 | 0.0000000000 |
| H | 3.7082246113 | 2.4885986669 | 0.0000000000 |
| H | 1.2352994928 | 2.4901233578 | 0.0000000000 |
| H | -1.2352994928 | 2.4901233578 | 0.0000000000 |
| H | -3.7082246113 | 2.4885986669 | 0.0000000000 |
| H | -6.1915665383 | 2.4876672716 | 0.0000000000 |
| H | -8.3302360217 | 1.2457864743 | 0.0000000000 |
| H | 8.3302360217 | -1.2457864743 | 0.0000000000 |
| H | 6.1915665383 | -2.4876672716 | 0.0000000000 |
| H | 3.7082246113 | -2.4885986669 | 0.0000000000 |
| H | 1.2352994928 | -2.4901233578 | 0.0000000000 |
| H | -1.2352994928 | -2.4901233578 | 0.0000000000 |
| H | -3.7082246113 | -2.4885986669 | 0.0000000000 |
| H | -6.1915665383 | -2.4876672716 | 0.0000000000 |
| H | -8.3302360217 | -1.2457864743 | 0.0000000000 |

**heptacene (singlet)**

48
Energy: -1147.16415 hartree

| | | | |
|---|---|---|---|
| C | 8.6122767702 | 0.7122696444 | 0.0000000000 |
| C | 7.4188181320 | 1.4082806814 | 0.0000000000 |
| C | 6.1675262806 | 0.7210550834 | 0.0000000000 |
| C | 4.9386981587 | 1.4075604258 | 0.0000000000 |

| | | | |
|---|---|---|---|
| C | 3.7041676096 | 0.7240581734 | 0.0000000000 |
| C | 2.4679359051 | 1.4091887277 | 0.0000000000 |
| C | 1.2352797353 | 0.7255836377 | 0.0000000000 |
| C | 0.0000000000 | 1.4095265890 | 0.0000000000 |
| C | -1.2352797353 | 0.7255836377 | 0.0000000000 |
| C | -2.4679359051 | 1.4091887277 | 0.0000000000 |
| C | -3.7041676096 | 0.7240581734 | 0.0000000000 |
| C | -4.9386981587 | 1.4075604258 | 0.0000000000 |
| C | -6.1675262806 | 0.7210550834 | 0.0000000000 |
| C | -7.4188181320 | 1.4082806814 | 0.0000000000 |
| C | -8.6122767702 | 0.7122696444 | 0.0000000000 |
| C | 8.6122767702 | -0.7122696444 | 0.0000000000 |
| C | 7.4188181320 | -1.4082806814 | 0.0000000000 |
| C | 6.1675262806 | -0.7210550834 | 0.0000000000 |
| C | 4.9386981587 | -1.4075604258 | 0.0000000000 |
| C | 3.7041676096 | -0.7240581734 | 0.0000000000 |
| C | 2.4679359051 | -1.4091887277 | 0.0000000000 |
| C | 1.2352797353 | -0.7255836377 | 0.0000000000 |
| C | 0.0000000000 | -1.4095265890 | 0.0000000000 |
| C | -1.2352797353 | -0.7255836377 | 0.0000000000 |
| C | -2.4679359051 | -1.4091887277 | 0.0000000000 |
| C | -3.7041676096 | -0.7240581734 | 0.0000000000 |
| C | -4.9386981587 | -1.4075604258 | 0.0000000000 |
| C | -6.1675262806 | -0.7210550834 | 0.0000000000 |
| C | -7.4188181320 | -1.4082806814 | 0.0000000000 |
| C | -8.6122767702 | -0.7122696444 | 0.0000000000 |
| H | 9.5522672947 | 1.2473800763 | 0.0000000000 |
| H | 7.4200268851 | 2.4905117146 | 0.0000000000 |
| H | 4.9396420277 | 2.4899720350 | 0.0000000000 |
| H | 2.4683551970 | 2.4914560346 | 0.0000000000 |
| H | 0.0000000000 | 2.4917749074 | 0.0000000000 |
| H | -2.4683551970 | 2.4914560346 | 0.0000000000 |
| H | -4.9396420277 | 2.4899720350 | 0.0000000000 |
| H | -7.4200268851 | 2.4905117146 | 0.0000000000 |
| H | -9.5522672947 | 1.2473800763 | 0.0000000000 |
| H | 9.5522672947 | -1.2473800763 | 0.0000000000 |
| H | 7.4200268851 | -2.4905117146 | 0.0000000000 |
| H | 4.9396420277 | -2.4899720350 | 0.0000000000 |
| H | 2.4683551970 | -2.4914560346 | 0.0000000000 |
| H | 0.0000000000 | -2.4917749074 | 0.0000000000 |
| H | -2.4683551970 | -2.4914560346 | 0.0000000000 |
| H | -4.9396420277 | -2.4899720350 | 0.0000000000 |
| H | -7.4200268851 | -2.4905117146 | 0.0000000000 |
| H | -9.5522672947 | -1.2473800763 | 0.0000000000 |

**heptacene (triplet)**

```
48
Energy: -1147.14083 hartree
  C      8.6235901121      0.7087414463      0.0000000000
  C      7.4239432432      1.4062101190      0.0000000000
  C      6.1784085580      0.7193564533      0.0000000000
  C      4.9418979411      1.4065135615      0.0000000000
  C      3.7109065333      0.7233165900      0.0000000000
  C      2.4699100159      1.4080517995      0.0000000000
  C      1.2373299917      0.7246659830      0.0000000000
  C      0.0000000000      1.4081757951      0.0000000000
  C     -1.2373299917      0.7246659830      0.0000000000
  C     -2.4699100159      1.4080517995      0.0000000000
  C     -3.7109065333      0.7233165900      0.0000000000
  C     -4.9418979411      1.4065135615      0.0000000000
  C     -6.1784085580      0.7193564533      0.0000000000
  C     -7.4239432432      1.4062101190      0.0000000000
  C     -8.6235901121      0.7087414463      0.0000000000
  C      8.6235901121     -0.7087414463      0.0000000000
  C      7.4239432432     -1.4062101190      0.0000000000
  C      6.1784085580     -0.7193564533      0.0000000000
  C      4.9418979411     -1.4065135615      0.0000000000
  C      3.7109065333     -0.7233165900      0.0000000000
  C      2.4699100159     -1.4080517995      0.0000000000
  C      1.2373299917     -0.7246659830      0.0000000000
  C      0.0000000000     -1.4081757951      0.0000000000
  C     -1.2373299917     -0.7246659830      0.0000000000
  C     -2.4699100159     -1.4080517995      0.0000000000
  C     -3.7109065333     -0.7233165900      0.0000000000
  C     -4.9418979411     -1.4065135615      0.0000000000
  C     -6.1784085580     -0.7193564533      0.0000000000
  C     -7.4239432432     -1.4062101190      0.0000000000
  C     -8.6235901121     -0.7087414463      0.0000000000
  H      9.5621667217      1.2462569976      0.0000000000
  H      7.4255028583      2.4884317733      0.0000000000
  H      4.9429938700      2.4889034676      0.0000000000
  H      2.4702227187      2.4903181846      0.0000000000
  H      0.0000000000      2.4904410786      0.0000000000
  H     -2.4702227187      2.4903181846      0.0000000000
  H     -4.9429938700      2.4889034676      0.0000000000
  H     -7.4255028583      2.4884317733      0.0000000000
  H     -9.5621667217      1.2462569976      0.0000000000
  H      9.5621667217     -1.2462569976      0.0000000000
  H      7.4255028583     -2.4884317733      0.0000000000
```

```
  H      4.9429938700     -2.4889034676      0.0000000000
  H      2.4702227187     -2.4903181846      0.0000000000
  H      0.0000000000     -2.4904410786      0.0000000000
  H     -2.4702227187     -2.4903181846      0.0000000000
  H     -4.9429938700     -2.4889034676      0.0000000000
  H     -7.4255028583     -2.4884317733      0.0000000000
  H     -9.5621667217     -1.2462569976      0.0000000000
```

**octacene (singlet)**

```
54
Energy: -1299.89165 hartree
  C      9.8474254155      0.7119978808      0.0000000000
  C      8.6535683982      1.4080640581      0.0000000000
  C      7.4028120666      0.7207808499      0.0000000000
  C      6.1731565621      1.4073335467      0.0000000000
  C      4.9396171468      0.7238102394      0.0000000000
  C      3.7020228203      1.4089263335      0.0000000000
  C      2.4708747229      0.7254284242      0.0000000000
  C      1.2337761633      1.4092569064      0.0000000000
  C      0.0000000000      0.7257936178      0.0000000000
  C     -1.2337761633      1.4092569064      0.0000000000
  C     -2.4708747229      0.7254284242      0.0000000000
  C     -3.7020228203      1.4089263335      0.0000000000
  C     -4.9396171468      0.7238102394      0.0000000000
  C     -6.1731565621      1.4073335467      0.0000000000
  C     -7.4028120666      0.7207808499      0.0000000000
  C     -8.6535683982      1.4080640581      0.0000000000
  C     -9.8474254155      0.7119978808      0.0000000000
  C      9.8474254155     -0.7119978808      0.0000000000
  C      8.6535683982     -1.4080640581      0.0000000000
  C      7.4028120666     -0.7207808499      0.0000000000
  C      6.1731565621     -1.4073335467      0.0000000000
  C      4.9396171468     -0.7238102394      0.0000000000
  C      3.7020228203     -1.4089263335      0.0000000000
  C      2.4708747229     -0.7254284242      0.0000000000
  C      1.2337761633     -1.4092569064      0.0000000000
  C      0.0000000000     -0.7257936178      0.0000000000
  C     -1.2337761633     -1.4092569064      0.0000000000
  C     -2.4708747229     -0.7254284242      0.0000000000
  C     -3.7020228203     -1.4089263335      0.0000000000
  C     -4.9396171468     -0.7238102394      0.0000000000
  C     -6.1731565621     -1.4073335467      0.0000000000
  C     -7.4028120666     -0.7207808499      0.0000000000
  C     -8.6535683982     -1.4080640581      0.0000000000
  C     -9.8474254155     -0.7119978808      0.0000000000
```

```
  H     10.7873154880      1.2472814126      0.0000000000
  H      8.6547588976      2.4902953435      0.0000000000
  H      6.1740844496      2.4897503415      0.0000000000
  H      3.7024338161      2.4912070517      0.0000000000
  H      1.2338532523      2.4915251976      0.0000000000
  H     -1.2338532523      2.4915251976      0.0000000000
  H     -3.7024338161      2.4912070517      0.0000000000
  H     -6.1740844496      2.4897503415      0.0000000000
  H     -8.6547588976      2.4902953435      0.0000000000
  H    -10.7873154880      1.2472814126      0.0000000000
  H     10.7873154880     -1.2472814126      0.0000000000
  H      8.6547588976     -2.4902953435      0.0000000000
  H      6.1740844496     -2.4897503415      0.0000000000
  H      3.7024338161     -2.4912070517      0.0000000000
  H      1.2338532523     -2.4915251976      0.0000000000
  H     -1.2338532523     -2.4915251976      0.0000000000
  H     -3.7024338161     -2.4912070517      0.0000000000
  H     -6.1740844496     -2.4897503415      0.0000000000
  H     -8.6547588976     -2.4902953435      0.0000000000
  H    -10.7873154880     -1.2472814126      0.0000000000
```

**octacene (triplet)**

```
54
Energy: -1299.87167 hartree
  C      9.8559563487      0.7096747908      0.0000000000
  C      8.6579992341      1.4067078309      0.0000000000
  C      7.4109948985      0.7197251791      0.0000000000
  C      6.1764423661      1.4067443804      0.0000000000
  C      4.9447261740      0.7234484663      0.0000000000
  C      3.7047197243      1.4082722873      0.0000000000
  C      2.4727439790      0.7246999098      0.0000000000
  C      1.2349201982      1.4082997956      0.0000000000
  C      0.0000000000      0.7247549238      0.0000000000
  C     -1.2349201982      1.4082997956      0.0000000000
  C     -2.4727439790      0.7246999098      0.0000000000
  C     -3.7047197243      1.4082722873      0.0000000000
  C     -4.9447261740      0.7234484663      0.0000000000
  C     -6.1764423661      1.4067443804      0.0000000000
  C     -7.4109948985      0.7197251791      0.0000000000
  C     -8.6579992341      1.4067078309      0.0000000000
  C     -9.8559563487      0.7096747908      0.0000000000
  C      9.8559563487     -0.7096747908      0.0000000000
  C      8.6579992341     -1.4067078309      0.0000000000
  C      7.4109948985     -0.7197251791      0.0000000000
  C      6.1764423661     -1.4067443804      0.0000000000
```

| | | | |
|---|---|---|---|
| C | 4.9447261740 | -0.7234484663 | 0.0000000000 |
| C | 3.7047197243 | -1.4082722873 | 0.0000000000 |
| C | 2.4727439790 | -0.7246999098 | 0.0000000000 |
| C | 1.2349201982 | -1.4082997956 | 0.0000000000 |
| C | 0.0000000000 | -0.7247549238 | 0.0000000000 |
| C | -1.2349201982 | -1.4082997956 | 0.0000000000 |
| C | -2.4727439790 | -0.7246999098 | 0.0000000000 |
| C | -3.7047197243 | -1.4082722873 | 0.0000000000 |
| C | -4.9447261740 | -0.7234484663 | 0.0000000000 |
| C | -6.1764423661 | -1.4067443804 | 0.0000000000 |
| C | -7.4109948985 | -0.7197251791 | 0.0000000000 |
| C | -8.6579992341 | -1.4067078309 | 0.0000000000 |
| C | -9.8559563487 | -0.7096747908 | 0.0000000000 |
| H | 10.7949097977 | 1.2465491927 | 0.0000000000 |
| H | 8.6594333599 | 2.4889321676 | 0.0000000000 |
| H | 6.1774987736 | 2.4891386763 | 0.0000000000 |
| H | 3.7050007116 | 2.4905415232 | 0.0000000000 |
| H | 1.2349084957 | 2.4905786580 | 0.0000000000 |
| H | -1.2349084957 | 2.4905786580 | 0.0000000000 |
| H | -3.7050007116 | 2.4905415232 | 0.0000000000 |
| H | -6.1774987736 | 2.4891386763 | 0.0000000000 |
| H | -8.6594333599 | 2.4889321676 | 0.0000000000 |
| H | -10.7949097977 | 1.2465491927 | 0.0000000000 |
| H | 10.7949097977 | -1.2465491927 | 0.0000000000 |
| H | 8.6594333599 | -2.4889321676 | 0.0000000000 |
| H | 6.1774987736 | -2.4891386763 | 0.0000000000 |
| H | 3.7050007116 | -2.4905415232 | 0.0000000000 |
| H | 1.2349084957 | -2.4905786580 | 0.0000000000 |
| H | -1.2349084957 | -2.4905786580 | 0.0000000000 |
| H | -3.7050007116 | -2.4905415232 | 0.0000000000 |
| H | -6.1774987736 | -2.4891386763 | 0.0000000000 |
| H | -8.6594333599 | -2.4889321676 | 0.0000000000 |
| H | -10.7949097977 | -1.2465491927 | 0.0000000000 |

**nonacene (singlet)**

60
Energy: -1452.61925 hartree

| | | | |
|---|---|---|---|
| C | 11.0821068718 | 0.7119331575 | 0.0000000000 |
| C | 9.8881817772 | 1.4079949146 | 0.0000000000 |
| C | 8.6375596643 | 0.7206730221 | 0.0000000000 |
| C | 7.4076831732 | 1.4072324892 | 0.0000000000 |
| C | 6.1745017655 | 0.7236659849 | 0.0000000000 |
| C | 4.9363702558 | 1.4087806470 | 0.0000000000 |
| C | 3.7060312372 | 0.7252593127 | 0.0000000000 |
| C | 2.4678171428 | 1.4090500242 | 0.0000000000 |

| | | | |
|---|---|---|---|
| C | 1.2354895461 | 0.7256806962 | 0.0000000000 |
| C | 0.0000000000 | 1.4090286305 | 0.0000000000 |
| C | -1.2354895461 | 0.7256806962 | 0.0000000000 |
| C | -2.4678171428 | 1.4090500242 | 0.0000000000 |
| C | -3.7060312372 | 0.7252593127 | 0.0000000000 |
| C | -4.9363702558 | 1.4087806470 | 0.0000000000 |
| C | -6.1745017655 | 0.7236659849 | 0.0000000000 |
| C | -7.4076831732 | 1.4072324892 | 0.0000000000 |
| C | -8.6375596643 | 0.7206730221 | 0.0000000000 |
| C | -9.8881817772 | 1.4079949146 | 0.0000000000 |
| C | -11.0821068718 | 0.7119331575 | 0.0000000000 |
| C | 11.0821068718 | -0.7119331575 | 0.0000000000 |
| C | 9.8881817772 | -1.4079949146 | 0.0000000000 |
| C | 8.6375596643 | -0.7206730221 | 0.0000000000 |
| C | 7.4076831732 | -1.4072324892 | 0.0000000000 |
| C | 6.1745017655 | -0.7236659849 | 0.0000000000 |
| C | 4.9363702558 | -1.4087806470 | 0.0000000000 |
| C | 3.7060312372 | -0.7252593127 | 0.0000000000 |
| C | 2.4678171428 | -1.4090500242 | 0.0000000000 |
| C | 1.2354895461 | -0.7256806962 | 0.0000000000 |
| C | 0.0000000000 | -1.4090286305 | 0.0000000000 |
| C | -1.2354895461 | -0.7256806962 | 0.0000000000 |
| C | -2.4678171428 | -1.4090500242 | 0.0000000000 |
| C | -3.7060312372 | -0.7252593127 | 0.0000000000 |
| C | -4.9363702558 | -1.4087806470 | 0.0000000000 |
| C | -6.1745017655 | -0.7236659849 | 0.0000000000 |
| C | -7.4076831732 | -1.4072324892 | 0.0000000000 |
| C | -8.6375596643 | -0.7206730221 | 0.0000000000 |
| C | -9.8881817772 | -1.4079949146 | 0.0000000000 |
| C | -11.0821068718 | -0.7119331575 | 0.0000000000 |
| H | 12.0219761088 | 1.2472521695 | 0.0000000000 |
| H | 9.8893503817 | 2.4902258251 | 0.0000000000 |
| H | 7.4085910401 | 2.4896503968 | 0.0000000000 |
| H | 4.9367573376 | 2.4910672041 | 0.0000000000 |
| H | 2.4678802253 | 2.4913320963 | 0.0000000000 |
| H | 0.0000000000 | 2.4913173152 | 0.0000000000 |
| H | -2.4678802253 | 2.4913320963 | 0.0000000000 |
| H | -4.9367573376 | 2.4910672041 | 0.0000000000 |
| H | -7.4085910401 | 2.4896503968 | 0.0000000000 |
| H | -9.8893503817 | 2.4902258251 | 0.0000000000 |
| H | -12.0219761088 | 1.2472521695 | 0.0000000000 |
| H | 12.0219761088 | -1.2472521695 | 0.0000000000 |
| H | 9.8893503817 | -2.4902258251 | 0.0000000000 |
| H | 7.4085910401 | -2.4896503968 | 0.0000000000 |
| H | 4.9367573376 | -2.4910672041 | 0.0000000000 |

| | | | |
|---|---|---|---|
| H | 2.4678802253 | -2.4913320963 | 0.0000000000 |
| H | 0.0000000000 | -2.4913173152 | 0.0000000000 |
| H | -2.4678802253 | -2.4913320963 | 0.0000000000 |
| H | -4.9367573376 | -2.4910672041 | 0.0000000000 |
| H | -7.4085910401 | -2.4896503968 | 0.0000000000 |
| H | -9.8893503817 | -2.4902258251 | 0.0000000000 |
| H | -12.0219761088 | -1.2472521695 | 0.0000000000 |

**nonacene (triplet)**

60
Energy: -1452.60166 hartree

| | | | |
|---|---|---|---|
| C | 11.0890424031 | 0.7102428473 | 0.0000000000 |
| C | 9.8921001196 | 1.4070186392 | 0.0000000000 |
| C | 8.6442105544 | 0.7199567494 | 0.0000000000 |
| C | 7.4108338875 | 1.4068821502 | 0.0000000000 |
| C | 6.1786898362 | 0.7235539563 | 0.0000000000 |
| C | 4.9393304897 | 1.4084425675 | 0.0000000000 |
| C | 3.7074901695 | 0.7248308046 | 0.0000000000 |
| C | 2.4698303332 | 1.4084494529 | 0.0000000000 |
| C | 1.2356870354 | 0.7247526596 | 0.0000000000 |
| C | 0.0000000000 | 1.4083009653 | 0.0000000000 |
| C | -1.2356870354 | 0.7247526596 | 0.0000000000 |
| C | -2.4698303332 | 1.4084494529 | 0.0000000000 |
| C | -3.7074901695 | 0.7248308046 | 0.0000000000 |
| C | -4.9393304897 | 1.4084425675 | 0.0000000000 |
| C | -6.1786898362 | 0.7235539563 | 0.0000000000 |
| C | -7.4108338875 | 1.4068821502 | 0.0000000000 |
| C | -8.6442105544 | 0.7199567494 | 0.0000000000 |
| C | -9.8921001196 | 1.4070186392 | 0.0000000000 |
| C | -11.0890424031 | 0.7102428473 | 0.0000000000 |
| C | 11.0890424031 | -0.7102428473 | 0.0000000000 |
| C | 9.8921001196 | -1.4070186392 | 0.0000000000 |
| C | 8.6442105544 | -0.7199567494 | 0.0000000000 |
| C | 7.4108338875 | -1.4068821502 | 0.0000000000 |
| C | 6.1786898362 | -0.7235539563 | 0.0000000000 |
| C | 4.9393304897 | -1.4084425675 | 0.0000000000 |
| C | 3.7074901695 | -0.7248308046 | 0.0000000000 |
| C | 2.4698303332 | -1.4084494529 | 0.0000000000 |
| C | 1.2356870354 | -0.7247526596 | 0.0000000000 |
| C | 0.0000000000 | -1.4083009653 | 0.0000000000 |
| C | -1.2356870354 | -0.7247526596 | 0.0000000000 |
| C | -2.4698303332 | -1.4084494529 | 0.0000000000 |
| C | -3.7074901695 | -0.7248308046 | 0.0000000000 |
| C | -4.9393304897 | -1.4084425675 | 0.0000000000 |
| C | -6.1786898362 | -0.7235539563 | 0.0000000000 |

| | | | |
|---|---|---|---|
| C | -7.4108338875 | -1.4068821502 | 0.0000000000 |
| C | -8.6442105544 | -0.7199567494 | 0.0000000000 |
| C | -9.8921001196 | -1.4070186392 | 0.0000000000 |
| C | -11.0890424031 | -0.7102428473 | 0.0000000000 |
| H | 12.0282241614 | 1.2467274868 | 0.0000000000 |
| H | 9.8934592792 | 2.4892442387 | 0.0000000000 |
| H | 7.4118718000 | 2.4892797566 | 0.0000000000 |
| H | 4.9396228106 | 2.4907111265 | 0.0000000000 |
| H | 2.4697658056 | 2.4907298253 | 0.0000000000 |
| H | 0.0000000000 | 2.4905964466 | 0.0000000000 |
| H | -2.4697658056 | 2.4907298253 | 0.0000000000 |
| H | -4.9396228106 | 2.4907111265 | 0.0000000000 |
| H | -7.4118718000 | 2.4892797566 | 0.0000000000 |
| H | -9.8934592792 | 2.4892442387 | 0.0000000000 |
| H | -12.0282241614 | 1.2467274868 | 0.0000000000 |
| H | 12.0282241614 | -1.2467274868 | 0.0000000000 |
| H | 9.8934592792 | -2.4892442387 | 0.0000000000 |
| H | 7.4118718000 | -2.4892797566 | 0.0000000000 |
| H | 4.9396228106 | -2.4907111265 | 0.0000000000 |
| H | 2.4697658056 | -2.4907298253 | 0.0000000000 |
| H | 0.0000000000 | -2.4905964466 | 0.0000000000 |
| H | -2.4697658056 | -2.4907298253 | 0.0000000000 |
| H | -4.9396228106 | -2.4907111265 | 0.0000000000 |
| H | -7.4118718000 | -2.4892797566 | 0.0000000000 |
| H | -9.8934592792 | -2.4892442387 | 0.0000000000 |
| H | -12.0282241614 | -1.2467274868 | 0.0000000000 |

**decacene (singlet)**

66
Energy: -1605.34686 hartree

| | | | |
|---|---|---|---|
| C | 12.3165568948 | 0.7119545937 | 0.0000000000 |
| C | 11.1226864448 | 1.4079970278 | 0.0000000000 |
| C | 9.8720346754 | 0.7206594760 | 0.0000000000 |
| C | 8.6421966466 | 1.4072089854 | 0.0000000000 |
| C | 7.4090549098 | 0.7236136091 | 0.0000000000 |
| C | 6.1708434972 | 1.4087276878 | 0.0000000000 |
| C | 4.9407650926 | 0.7251578523 | 0.0000000000 |
| C | 3.7021362591 | 1.4089470997 | 0.0000000000 |
| C | 2.4705635971 | 0.7255368945 | 0.0000000000 |
| C | 1.2340303457 | 1.4088561708 | 0.0000000000 |
| C | 0.0000000000 | 0.7255861114 | 0.0000000000 |
| C | -1.2340303457 | 1.4088561708 | 0.0000000000 |
| C | -2.4705635971 | 0.7255368945 | 0.0000000000 |
| C | -3.7021362591 | 1.4089470997 | 0.0000000000 |
| C | -4.9407650926 | 0.7251578523 | 0.0000000000 |

| | | | |
|---|---|---|---|
| C | -6.1708434972 | 1.4087276878 | 0.0000000000 |
| C | -7.4090549098 | 0.7236136091 | 0.0000000000 |
| C | -8.6421966466 | 1.4072089854 | 0.0000000000 |
| C | -9.8720346754 | 0.7206594760 | 0.0000000000 |
| C | -11.1226864448 | 1.4079970278 | 0.0000000000 |
| C | -12.3165568948 | 0.7119545937 | 0.0000000000 |
| C | 12.3165568948 | -0.7119545937 | 0.0000000000 |
| C | 11.1226864448 | -1.4079970278 | 0.0000000000 |
| C | 9.8720346754 | -0.7206594760 | 0.0000000000 |
| C | 8.6421966466 | -1.4072089854 | 0.0000000000 |
| C | 7.4090549098 | -0.7236136091 | 0.0000000000 |
| C | 6.1708434972 | -1.4087276878 | 0.0000000000 |
| C | 4.9407650926 | -0.7251578523 | 0.0000000000 |
| C | 3.7021362591 | -1.4089470997 | 0.0000000000 |
| C | 2.4705635971 | -0.7255368945 | 0.0000000000 |
| C | 1.2340303457 | -1.4088561708 | 0.0000000000 |
| C | 0.0000000000 | -0.7255861114 | 0.0000000000 |
| C | -1.2340303457 | -1.4088561708 | 0.0000000000 |
| C | -2.4705635971 | -0.7255368945 | 0.0000000000 |
| C | -3.7021362591 | -1.4089470997 | 0.0000000000 |
| C | -4.9407650926 | -0.7251578523 | 0.0000000000 |
| C | -6.1708434972 | -1.4087276878 | 0.0000000000 |
| C | -7.4090549098 | -0.7236136091 | 0.0000000000 |
| C | -8.6421966466 | -1.4072089854 | 0.0000000000 |
| C | -9.8720346754 | -0.7206594760 | 0.0000000000 |
| C | -11.1226864448 | -1.4079970278 | 0.0000000000 |
| C | -12.3165568948 | -0.7119545937 | 0.0000000000 |
| H | 13.2564357244 | 1.2472557521 | 0.0000000000 |
| H | 11.1238422013 | 2.4902272101 | 0.0000000000 |
| H | 8.6430912416 | 2.4896261176 | 0.0000000000 |
| H | 6.1712113888 | 2.4910149131 | 0.0000000000 |
| H | 3.7021717784 | 2.4912342228 | 0.0000000000 |
| H | 1.2340150220 | 2.4911577844 | 0.0000000000 |
| H | -1.2340150220 | 2.4911577844 | 0.0000000000 |
| H | -3.7021717784 | 2.4912342228 | 0.0000000000 |
| H | -6.1712113888 | 2.4910149131 | 0.0000000000 |
| H | -8.6430912416 | 2.4896261176 | 0.0000000000 |
| H | -11.1238422013 | 2.4902272101 | 0.0000000000 |
| H | -13.2564357244 | 1.2472557521 | 0.0000000000 |
| H | 13.2564357244 | -1.2472557521 | 0.0000000000 |
| H | 11.1238422013 | -2.4902272101 | 0.0000000000 |
| H | 8.6430912416 | -2.4896261176 | 0.0000000000 |
| H | 6.1712113888 | -2.4910149131 | 0.0000000000 |
| H | 3.7021717784 | -2.4912342228 | 0.0000000000 |
| H | 1.2340150220 | -2.4911577844 | 0.0000000000 |

| | | | |
|---|---|---|---|
| H | -1.2340150220 | -2.4911577844 | 0.0000000000 |
| H | -3.7021717784 | -2.4912342228 | 0.0000000000 |
| H | -6.1712113888 | -2.4910149131 | 0.0000000000 |
| H | -8.6430912416 | -2.4896261176 | 0.0000000000 |
| H | -11.1238422013 | -2.4902272101 | 0.0000000000 |
| H | -13.2564357244 | -1.2472557521 | 0.0000000000 |

**decacene (triplet)**

66
Energy: -1605.33110 hartree

| | | | |
|---|---|---|---|
| C | 12.3225678653 | 0.7106024320 | 0.0000000000 |
| C | 11.1262712433 | 1.4072142820 | 0.0000000000 |
| C | 9.8778303405 | 0.7200965591 | 0.0000000000 |
| C | 8.6451712703 | 1.4069538397 | 0.0000000000 |
| C | 7.4128396763 | 0.7236027180 | 0.0000000000 |
| C | 6.1737851873 | 1.4085416840 | 0.0000000000 |
| C | 4.9421177054 | 0.7249614594 | 0.0000000000 |
| C | 3.7045867553 | 1.4085837410 | 0.0000000000 |
| C | 2.4706444125 | 0.7248526537 | 0.0000000000 |
| C | 1.2350038073 | 1.4083481203 | 0.0000000000 |
| C | 0.0000000000 | 0.7246665646 | 0.0000000000 |
| C | -1.2350038073 | 1.4083481203 | 0.0000000000 |
| C | -2.4706444125 | 0.7248526537 | 0.0000000000 |
| C | -3.7045867553 | 1.4085837410 | 0.0000000000 |
| C | -4.9421177054 | 0.7249614594 | 0.0000000000 |
| C | -6.1737851873 | 1.4085416840 | 0.0000000000 |
| C | -7.4128396763 | 0.7236027180 | 0.0000000000 |
| C | -8.6451712703 | 1.4069538397 | 0.0000000000 |
| C | -9.8778303405 | 0.7200965591 | 0.0000000000 |
| C | -11.1262712433 | 1.4072142820 | 0.0000000000 |
| C | -12.3225678653 | 0.7106024320 | 0.0000000000 |
| C | 12.3225678653 | -0.7106024320 | 0.0000000000 |
| C | 11.1262712433 | -1.4072142820 | 0.0000000000 |
| C | 9.8778303405 | -0.7200965591 | 0.0000000000 |
| C | 8.6451712703 | -1.4069538397 | 0.0000000000 |
| C | 7.4128396763 | -0.7236027180 | 0.0000000000 |
| C | 6.1737851873 | -1.4085416840 | 0.0000000000 |
| C | 4.9421177054 | -0.7249614594 | 0.0000000000 |
| C | 3.7045867553 | -1.4085837410 | 0.0000000000 |
| C | 2.4706444125 | -0.7248526537 | 0.0000000000 |
| C | 1.2350038073 | -1.4083481203 | 0.0000000000 |
| C | 0.0000000000 | -0.7246665646 | 0.0000000000 |
| C | -1.2350038073 | -1.4083481203 | 0.0000000000 |
| C | -2.4706444125 | -0.7248526537 | 0.0000000000 |
| C | -3.7045867553 | -1.4085837410 | 0.0000000000 |

| | | | |
|---|---|---|---|
| C | -4.9421177054 | -0.7249614594 | 0.0000000000 |
| C | -6.1737851873 | -1.4085416840 | 0.0000000000 |
| C | -7.4128396763 | -0.7236027180 | 0.0000000000 |
| C | -8.6451712703 | -1.4069538397 | 0.0000000000 |
| C | -9.8778303405 | -0.7200965591 | 0.0000000000 |
| C | -11.1262712433 | -1.4072142820 | 0.0000000000 |
| C | -12.3225678653 | -0.7106024320 | 0.0000000000 |
| H | 13.2618902584 | 1.2468462570 | 0.0000000000 |
| H | 11.1275876701 | 2.4894410134 | 0.0000000000 |
| H | 8.6461912995 | 2.4893542127 | 0.0000000000 |
| H | 6.1741138298 | 2.4908101985 | 0.0000000000 |
| H | 3.7045221716 | 2.4908616376 | 0.0000000000 |
| H | 1.2349422215 | 2.4906486121 | 0.0000000000 |
| H | -1.2349422215 | 2.4906486121 | 0.0000000000 |
| H | -3.7045221716 | 2.4908616376 | 0.0000000000 |
| H | -6.1741138298 | 2.4908101985 | 0.0000000000 |
| H | -8.6461912995 | 2.4893542127 | 0.0000000000 |
| H | -11.1275876701 | 2.4894410134 | 0.0000000000 |
| H | -13.2618902584 | 1.2468462570 | 0.0000000000 |
| H | 13.2618902584 | -1.2468462570 | 0.0000000000 |
| H | 11.1275876701 | -2.4894410134 | 0.0000000000 |
| H | 8.6461912995 | -2.4893542127 | 0.0000000000 |
| H | 6.1741138298 | -2.4908101985 | 0.0000000000 |
| H | 3.7045221716 | -2.4908616376 | 0.0000000000 |
| H | 1.2349422215 | -2.4906486121 | 0.0000000000 |
| H | -1.2349422215 | -2.4906486121 | 0.0000000000 |
| H | -3.7045221716 | -2.4908616376 | 0.0000000000 |
| H | -6.1741138298 | -2.4908101985 | 0.0000000000 |
| H | -8.6461912995 | -2.4893542127 | 0.0000000000 |
| H | -11.1275876701 | -2.4894410134 | 0.0000000000 |
| H | -13.2618902584 | -1.2468462570 | 0.0000000000 |

**undecacene (singlet)**

72
Energy: -1758.07442 hartree

| | | | |
|---|---|---|---|
| C | 13.5509273819 | 0.7119942831 | 0.0000000000 |
| C | 12.3571301010 | 1.4080221427 | 0.0000000000 |
| C | 11.1064109052 | 0.7206824460 | 0.0000000000 |
| C | 9.8766778460 | 1.4072203776 | 0.0000000000 |
| C | 8.6434661806 | 0.7236129244 | 0.0000000000 |
| C | 7.4053451992 | 1.4087251422 | 0.0000000000 |
| C | 6.1752661783 | 0.7251217619 | 0.0000000000 |
| C | 4.9366033052 | 1.4089173937 | 0.0000000000 |
| C | 3.7052605488 | 0.7254439400 | 0.0000000000 |
| C | 2.4683449640 | 1.4087722169 | 0.0000000000 |

| | | | |
|---|---|---|---|
| C | 1.2350612714 | 0.7254473663 | 0.0000000000 |
| C | 0.0000000000 | 1.4087013666 | 0.0000000000 |
| C | -1.2350612714 | 0.7254473663 | 0.0000000000 |
| C | -2.4683449640 | 1.4087722169 | 0.0000000000 |
| C | -3.7052605488 | 0.7254439400 | 0.0000000000 |
| C | -4.9366033052 | 1.4089173937 | 0.0000000000 |
| C | -6.1752661783 | 0.7251217619 | 0.0000000000 |
| C | -7.4053451992 | 1.4087251422 | 0.0000000000 |
| C | -8.6434661806 | 0.7236129244 | 0.0000000000 |
| C | -9.8766778460 | 1.4072203776 | 0.0000000000 |
| C | -11.1064109052 | 0.7206824460 | 0.0000000000 |
| C | -12.3571301010 | 1.4080221427 | 0.0000000000 |
| C | -13.5509273819 | 0.7119942831 | 0.0000000000 |
| C | 13.5509273819 | -0.7119942831 | 0.0000000000 |
| C | 12.3571301010 | -1.4080221427 | 0.0000000000 |
| C | 11.1064109052 | -0.7206824460 | 0.0000000000 |
| C | 9.8766778460 | -1.4072203776 | 0.0000000000 |
| C | 8.6434661806 | -0.7236129244 | 0.0000000000 |
| C | 7.4053451992 | -1.4087251422 | 0.0000000000 |
| C | 6.1752661783 | -0.7251217619 | 0.0000000000 |
| C | 4.9366033052 | -1.4089173937 | 0.0000000000 |
| C | 3.7052605488 | -0.7254439400 | 0.0000000000 |
| C | 2.4683449640 | -1.4087722169 | 0.0000000000 |
| C | 1.2350612714 | -0.7254473663 | 0.0000000000 |
| C | 0.0000000000 | -1.4087013666 | 0.0000000000 |
| C | -1.2350612714 | -0.7254473663 | 0.0000000000 |
| C | -2.4683449640 | -1.4087722169 | 0.0000000000 |
| C | -3.7052605488 | -0.7254439400 | 0.0000000000 |
| C | -4.9366033052 | -1.4089173937 | 0.0000000000 |
| C | -6.1752661783 | -0.7251217619 | 0.0000000000 |
| C | -7.4053451992 | -1.4087251422 | 0.0000000000 |
| C | -8.6434661806 | -0.7236129244 | 0.0000000000 |
| C | -9.8766778460 | -1.4072203776 | 0.0000000000 |
| C | -11.1064109052 | -0.7206824460 | 0.0000000000 |
| C | -12.3571301010 | -1.4080221427 | 0.0000000000 |
| C | -13.5509273819 | -0.7119942831 | 0.0000000000 |
| H | 14.4908215838 | 1.2472670358 | 0.0000000000 |
| H | 12.3582811535 | 2.4902513502 | 0.0000000000 |
| H | 9.8775664466 | 2.4896360987 | 0.0000000000 |
| H | 7.4057026136 | 2.4910109005 | 0.0000000000 |
| H | 4.9366173689 | 2.4912043294 | 0.0000000000 |
| H | 2.4683009038 | 2.4910780905 | 0.0000000000 |
| H | 0.0000000000 | 2.4910151047 | 0.0000000000 |
| H | -2.4683009038 | 2.4910780905 | 0.0000000000 |
| H | -4.9366173689 | 2.4912043294 | 0.0000000000 |

| | | | |
|---|---|---|---|
| H | -7.4057026136 | 2.4910109005 | 0.0000000000 |
| H | -9.8775664466 | 2.4896360987 | 0.0000000000 |
| H | -12.3582811535 | 2.4902513502 | 0.0000000000 |
| H | -14.4908215838 | 1.2472670358 | 0.0000000000 |
| H | 14.4908215838 | -1.2472670358 | 0.0000000000 |
| H | 12.3582811535 | -2.4902513502 | 0.0000000000 |
| H | 9.8775664466 | -2.4896360987 | 0.0000000000 |
| H | 7.4057026136 | -2.4910109005 | 0.0000000000 |
| H | 4.9366173689 | -2.4912043294 | 0.0000000000 |
| H | 2.4683009038 | -2.4910780905 | 0.0000000000 |
| H | 0.0000000000 | -2.4910151047 | 0.0000000000 |
| H | -2.4683009038 | -2.4910780905 | 0.0000000000 |
| H | -4.9366173689 | -2.4912043294 | 0.0000000000 |
| H | -7.4057026136 | -2.4910109005 | 0.0000000000 |
| H | -9.8775664466 | -2.4896360987 | 0.0000000000 |
| H | -12.3582811535 | -2.4902513502 | 0.0000000000 |
| H | -14.4908215838 | -1.2472670358 | 0.0000000000 |

**undecacene (triplet)**

72
Energy: -1758.06019 hartree

| | | | |
|---|---|---|---|
| C | 13.5563309546 | 0.7108551028 | 0.0000000000 |
| C | 12.3604943692 | 1.4073518337 | 0.0000000000 |
| C | 11.1116645040 | 0.7201876489 | 0.0000000000 |
| C | 9.8794990313 | 1.4069929512 | 0.0000000000 |
| C | 8.6470818686 | 0.7236146144 | 0.0000000000 |
| C | 7.4081535502 | 1.4085899427 | 0.0000000000 |
| C | 6.1767462000 | 0.7250479172 | 0.0000000000 |
| C | 4.9391640982 | 1.4086797932 | 0.0000000000 |
| C | 3.7053994838 | 0.7249920166 | 0.0000000000 |
| C | 2.4699123247 | 1.4084273660 | 0.0000000000 |
| C | 1.2349498631 | 0.7246925157 | 0.0000000000 |
| C | 0.0000000000 | 1.4083147056 | 0.0000000000 |
| C | -1.2349498631 | 0.7246925157 | 0.0000000000 |
| C | -2.4699123247 | 1.4084273660 | 0.0000000000 |
| C | -3.7053994838 | 0.7249920166 | 0.0000000000 |
| C | -4.9391640982 | 1.4086797932 | 0.0000000000 |
| C | -6.1767462000 | 0.7250479172 | 0.0000000000 |
| C | -7.4081535502 | 1.4085899427 | 0.0000000000 |
| C | -8.6470818686 | 0.7236146144 | 0.0000000000 |
| C | -9.8794990313 | 1.4069929512 | 0.0000000000 |
| C | -11.1116645040 | 0.7201876489 | 0.0000000000 |
| C | -12.3604943692 | 1.4073518337 | 0.0000000000 |
| C | -13.5563309546 | 0.7108551028 | 0.0000000000 |
| C | 13.5563309546 | -0.7108551028 | 0.0000000000 |

| | | | |
|---|---|---|---|
| C | 12.3604943692 | -1.4073518337 | 0.0000000000 |
| C | 11.1116645040 | -0.7201876489 | 0.0000000000 |
| C | 9.8794990313 | -1.4069929512 | 0.0000000000 |
| C | 8.6470818686 | -0.7236146144 | 0.0000000000 |
| C | 7.4081535502 | -1.4085899427 | 0.0000000000 |
| C | 6.1767462000 | -0.7250479172 | 0.0000000000 |
| C | 4.9391640982 | -1.4086797932 | 0.0000000000 |
| C | 3.7053994838 | -0.7249920166 | 0.0000000000 |
| C | 2.4699123247 | -1.4084273660 | 0.0000000000 |
| C | 1.2349498631 | -0.7246925157 | 0.0000000000 |
| C | 0.0000000000 | -1.4083147056 | 0.0000000000 |
| C | -1.2349498631 | -0.7246925157 | 0.0000000000 |
| C | -2.4699123247 | -1.4084273660 | 0.0000000000 |
| C | -3.7053994838 | -0.7249920166 | 0.0000000000 |
| C | -4.9391640982 | -1.4086797932 | 0.0000000000 |
| C | -6.1767462000 | -0.7250479172 | 0.0000000000 |
| C | -7.4081535502 | -1.4085899427 | 0.0000000000 |
| C | -8.6470818686 | -0.7236146144 | 0.0000000000 |
| C | -9.8794990313 | -1.4069929512 | 0.0000000000 |
| C | -11.1116645040 | -0.7201876489 | 0.0000000000 |
| C | -12.3604943692 | -1.4073518337 | 0.0000000000 |
| C | -13.5563309546 | -0.7108551028 | 0.0000000000 |
| H | 14.4957564683 | 1.2469226421 | 0.0000000000 |
| H | 12.3617742988 | 2.4895788794 | 0.0000000000 |
| H | 9.8805008873 | 2.4893958753 | 0.0000000000 |
| H | 7.4085024981 | 2.4908598871 | 0.0000000000 |
| H | 4.9391115532 | 2.4909556575 | 0.0000000000 |
| H | 2.4698162674 | 2.4907268504 | 0.0000000000 |
| H | 0.0000000000 | 2.4906235823 | 0.0000000000 |
| H | -2.4698162674 | 2.4907268504 | 0.0000000000 |
| H | -4.9391115532 | 2.4909556575 | 0.0000000000 |
| H | -7.4085024981 | 2.4908598871 | 0.0000000000 |
| H | -9.8805008873 | 2.4893958753 | 0.0000000000 |
| H | -12.3617742988 | 2.4895788794 | 0.0000000000 |
| H | -14.4957564683 | 1.2469226421 | 0.0000000000 |
| H | 14.4957564683 | -1.2469226421 | 0.0000000000 |
| H | 12.3617742988 | -2.4895788794 | 0.0000000000 |
| H | 9.8805008873 | -2.4893958753 | 0.0000000000 |
| H | 7.4085024981 | -2.4908598871 | 0.0000000000 |
| H | 4.9391115532 | -2.4909556575 | 0.0000000000 |
| H | 2.4698162674 | -2.4907268504 | 0.0000000000 |
| H | 0.0000000000 | -2.4906235823 | 0.0000000000 |
| H | -2.4698162674 | -2.4907268504 | 0.0000000000 |
| H | -4.9391115532 | -2.4909556575 | 0.0000000000 |
| H | -7.4085024981 | -2.4908598871 | 0.0000000000 |

| | | | |
|---|---|---|---|
| H | -9.8805008873 | -2.4893958753 | 0.0000000000 |
| H | -12.3617742988 | -2.4895788794 | 0.0000000000 |
| H | -14.4957564683 | -1.2469226421 | 0.0000000000 |

**dodecacene (singlet)**

78
Energy: -1910.80196 hartree

| | | | |
|---|---|---|---|
| C | 14.7853044500 | 0.7120234105 | 0.0000000000 |
| C | 13.5915579400 | 1.4080445235 | 0.0000000000 |
| C | 12.3407876162 | 0.7207083763 | 0.0000000000 |
| C | 11.1111401642 | 1.4072393104 | 0.0000000000 |
| C | 9.8778498334 | 0.7236304739 | 0.0000000000 |
| C | 8.6398432665 | 1.4087410146 | 0.0000000000 |
| C | 7.4096812462 | 0.7251219920 | 0.0000000000 |
| C | 6.1711196707 | 1.4089232613 | 0.0000000000 |
| C | 4.9397599452 | 0.7254052334 | 0.0000000000 |
| C | 3.7028195496 | 1.4087476285 | 0.0000000000 |
| C | 2.4697558689 | 0.7253486033 | 0.0000000000 |
| C | 1.2343162355 | 1.4086224344 | 0.0000000000 |
| C | 0.0000000000 | 0.7253039989 | 0.0000000000 |
| C | -1.2343162355 | 1.4086224344 | 0.0000000000 |
| C | -2.4697558689 | 0.7253486033 | 0.0000000000 |
| C | -3.7028195496 | 1.4087476285 | 0.0000000000 |
| C | -4.9397599452 | 0.7254052334 | 0.0000000000 |
| C | -6.1711196707 | 1.4089232613 | 0.0000000000 |
| C | -7.4096812462 | 0.7251219920 | 0.0000000000 |
| C | -8.6398432665 | 1.4087410146 | 0.0000000000 |
| C | -9.8778498334 | 0.7236304739 | 0.0000000000 |
| C | -11.1111401642 | 1.4072393104 | 0.0000000000 |
| C | -12.3407876162 | 0.7207083763 | 0.0000000000 |
| C | -13.5915579400 | 1.4080445235 | 0.0000000000 |
| C | -14.7853044500 | 0.7120234105 | 0.0000000000 |
| C | 14.7853044500 | -0.7120234105 | 0.0000000000 |
| C | 13.5915579400 | -1.4080445235 | 0.0000000000 |
| C | 12.3407876162 | -0.7207083763 | 0.0000000000 |
| C | 11.1111401642 | -1.4072393104 | 0.0000000000 |
| C | 9.8778498334 | -0.7236304739 | 0.0000000000 |
| C | 8.6398432665 | -1.4087410146 | 0.0000000000 |
| C | 7.4096812462 | -0.7251219920 | 0.0000000000 |
| C | 6.1711196707 | -1.4089232613 | 0.0000000000 |
| C | 4.9397599452 | -0.7254052334 | 0.0000000000 |
| C | 3.7028195496 | -1.4087476285 | 0.0000000000 |
| C | 2.4697558689 | -0.7253486033 | 0.0000000000 |
| C | 1.2343162355 | -1.4086224344 | 0.0000000000 |
| C | 0.0000000000 | -0.7253039989 | 0.0000000000 |

| | | | |
|---|---|---|---|
| C | -1.2343162355 | -1.4086224344 | 0.0000000000 |
| C | -2.4697558689 | -0.7253486033 | 0.0000000000 |
| C | -3.7028195496 | -1.4087476285 | 0.0000000000 |
| C | -4.9397599452 | -0.7254052334 | 0.0000000000 |
| C | -6.1711196707 | -1.4089232613 | 0.0000000000 |
| C | -7.4096812462 | -0.7251219920 | 0.0000000000 |
| C | -8.6398432665 | -1.4087410146 | 0.0000000000 |
| C | -9.8778498334 | -0.7236304739 | 0.0000000000 |
| C | -11.1111401642 | -1.4072393104 | 0.0000000000 |
| C | -12.3407876162 | -0.7207083763 | 0.0000000000 |
| C | -13.5915579400 | -1.4080445235 | 0.0000000000 |
| C | -14.7853044500 | -0.7120234105 | 0.0000000000 |
| H | 15.7252094268 | 1.2472756685 | 0.0000000000 |
| H | 13.5927087196 | 2.4902727757 | 0.0000000000 |
| H | 11.1120278432 | 2.4896535988 | 0.0000000000 |
| H | 8.6401966293 | 2.4910248636 | 0.0000000000 |
| H | 6.1711218115 | 2.4912081195 | 0.0000000000 |
| H | 3.7027529353 | 2.4910528172 | 0.0000000000 |
| H | 1.2342881367 | 2.4909398837 | 0.0000000000 |
| H | -1.2342881367 | 2.4909398837 | 0.0000000000 |
| H | -3.7027529353 | 2.4910528172 | 0.0000000000 |
| H | -6.1711218115 | 2.4912081195 | 0.0000000000 |
| H | -8.6401966293 | 2.4910248636 | 0.0000000000 |
| H | -11.1120278432 | 2.4896535988 | 0.0000000000 |
| H | -13.5927087196 | 2.4902727757 | 0.0000000000 |
| H | -15.7252094268 | 1.2472756685 | 0.0000000000 |
| H | 15.7252094268 | -1.2472756685 | 0.0000000000 |
| H | 13.5927087196 | -2.4902727757 | 0.0000000000 |
| H | 11.1120278432 | -2.4896535988 | 0.0000000000 |
| H | 8.6401966293 | -2.4910248636 | 0.0000000000 |
| H | 6.1711218115 | -2.4912081195 | 0.0000000000 |
| H | 3.7027529353 | -2.4910528172 | 0.0000000000 |
| H | 1.2342881367 | -2.4909398837 | 0.0000000000 |
| H | -1.2342881367 | -2.4909398837 | 0.0000000000 |
| H | -3.7027529353 | -2.4910528172 | 0.0000000000 |
| H | -6.1711218115 | -2.4912081195 | 0.0000000000 |
| H | -8.6401966293 | -2.4910248636 | 0.0000000000 |
| H | -11.1120278432 | -2.4896535988 | 0.0000000000 |
| H | -13.5927087196 | -2.4902727757 | 0.0000000000 |
| H | -15.7252094268 | -1.2472756685 | 0.0000000000 |

**dodecacene (triplet)**

78
Energy: -1910.78900 hartree

| | | | |
|---|---|---|---|
| C | 14.7902307616 | 0.7110462938 | 0.0000000000 |

| | | | |
|---|---|---|---|
| C | 13.5947447606 | 1.4074573999 | 0.0000000000 |
| C | 12.3456135999 | 0.7202559742 | 0.0000000000 |
| C | 11.1138283163 | 1.4070203807 | 0.0000000000 |
| C | 9.8813447524 | 0.7236106499 | 0.0000000000 |
| C | 8.6424902555 | 1.4086134079 | 0.0000000000 |
| C | 7.4113526354 | 0.7250905693 | 0.0000000000 |
| C | 6.1736132497 | 1.4087386477 | 0.0000000000 |
| C | 4.9401272263 | 0.7251106342 | 0.0000000000 |
| C | 3.7046395897 | 1.4085015989 | 0.0000000000 |
| C | 2.4696625846 | 0.7247935314 | 0.0000000000 |
| C | 1.2349839513 | 1.4083438003 | 0.0000000000 |
| C | 0.0000000000 | 0.7246427338 | 0.0000000000 |
| C | -1.2349839513 | 1.4083438003 | 0.0000000000 |
| C | -2.4696625846 | 0.7247935314 | 0.0000000000 |
| C | -3.7046395897 | 1.4085015989 | 0.0000000000 |
| C | -4.9401272263 | 0.7251106342 | 0.0000000000 |
| C | -6.1736132497 | 1.4087386477 | 0.0000000000 |
| C | -7.4113526354 | 0.7250905693 | 0.0000000000 |
| C | -8.6424902555 | 1.4086134079 | 0.0000000000 |
| C | -9.8813447524 | 0.7236106499 | 0.0000000000 |
| C | -11.1138283163 | 1.4070203807 | 0.0000000000 |
| C | -12.3456135999 | 0.7202559742 | 0.0000000000 |
| C | -13.5947447606 | 1.4074573999 | 0.0000000000 |
| C | -14.7902307616 | 0.7110462938 | 0.0000000000 |
| C | 14.7902307616 | -0.7110462938 | 0.0000000000 |
| C | 13.5947447606 | -1.4074573999 | 0.0000000000 |
| C | 12.3456135999 | -0.7202559742 | 0.0000000000 |
| C | 11.1138283163 | -1.4070203807 | 0.0000000000 |
| C | 9.8813447524 | -0.7236106499 | 0.0000000000 |
| C | 8.6424902555 | -1.4086134079 | 0.0000000000 |
| C | 7.4113526354 | -0.7250905693 | 0.0000000000 |
| C | 6.1736132497 | -1.4087386477 | 0.0000000000 |
| C | 4.9401272263 | -0.7251106342 | 0.0000000000 |
| C | 3.7046395897 | -1.4085015989 | 0.0000000000 |
| C | 2.4696625846 | -0.7247935314 | 0.0000000000 |
| C | 1.2349839513 | -1.4083438003 | 0.0000000000 |
| C | 0.0000000000 | -0.7246427338 | 0.0000000000 |
| C | -1.2349839513 | -1.4083438003 | 0.0000000000 |
| C | -2.4696625846 | -0.7247935314 | 0.0000000000 |
| C | -3.7046395897 | -1.4085015989 | 0.0000000000 |
| C | -4.9401272263 | -0.7251106342 | 0.0000000000 |
| C | -6.1736132497 | -1.4087386477 | 0.0000000000 |
| C | -7.4113526354 | -0.7250905693 | 0.0000000000 |
| C | -8.6424902555 | -1.4086134079 | 0.0000000000 |
| C | -9.8813447524 | -0.7236106499 | 0.0000000000 |

| | | | |
|---|---|---|---|
| C | -11.1138283163 | -1.4070203807 | 0.0000000000 |
| C | -12.3456135999 | -0.7202559742 | 0.0000000000 |
| C | -13.5947447606 | -1.4074573999 | 0.0000000000 |
| C | -14.7902307616 | -0.7110462938 | 0.0000000000 |
| H | 15.7297355461 | 1.2469789853 | 0.0000000000 |
| H | 13.5959965819 | 2.4896846660 | 0.0000000000 |
| H | 11.1148129970 | 2.4894251849 | 0.0000000000 |
| H | 8.6428500020 | 2.4908852535 | 0.0000000000 |
| H | 6.1735766451 | 2.4910140897 | 0.0000000000 |
| H | 3.7045349794 | 2.4907992179 | 0.0000000000 |
| H | 1.2349401716 | 2.4906536385 | 0.0000000000 |
| H | -1.2349401716 | 2.4906536385 | 0.0000000000 |
| H | -3.7045349794 | 2.4907992179 | 0.0000000000 |
| H | -6.1735766451 | 2.4910140897 | 0.0000000000 |
| H | -8.6428500020 | 2.4908852535 | 0.0000000000 |
| H | -11.1148129970 | 2.4894251849 | 0.0000000000 |
| H | -13.5959965819 | 2.4896846660 | 0.0000000000 |
| H | -15.7297355461 | 1.2469789853 | 0.0000000000 |
| H | 15.7297355461 | -1.2469789853 | 0.0000000000 |
| H | 13.5959965819 | -2.4896846660 | 0.0000000000 |
| H | 11.1148129970 | -2.4894251849 | 0.0000000000 |
| H | 8.6428500020 | -2.4908852535 | 0.0000000000 |
| H | 6.1735766451 | -2.4910140897 | 0.0000000000 |
| H | 3.7045349794 | -2.4907992179 | 0.0000000000 |
| H | 1.2349401716 | -2.4906536385 | 0.0000000000 |
| H | -1.2349401716 | -2.4906536385 | 0.0000000000 |
| H | -3.7045349794 | -2.4907992179 | 0.0000000000 |
| H | -6.1735766451 | -2.4910140897 | 0.0000000000 |
| H | -8.6428500020 | -2.4908852535 | 0.0000000000 |
| H | -11.1148129970 | -2.4894251849 | 0.0000000000 |
| H | -13.5959965819 | -2.4896846660 | 0.0000000000 |
| H | -15.7297355461 | -1.2469789853 | 0.0000000000 |
